# Supplementary material for: ZK-GanDef: A GAN based Zero Knowledge Adversarial Training Defense for Neural Networks
Source: arXiv:1904.08516 source file (2019-04-17)
Supplement: Supplementary file 1 [file appendix.tex]

\begin{appendices}
\balance

\section{Structures and Training Settings of Neural Networks} \label{appendix:tables}

\begin{table}[H]
    \begin{center}
    \begin{tabular}{c | c | c | c | c }
    \hline \hline
    Layer & Kernel Size & Strides & Padding & Init \\
    \hline \hline
    Convolution & $5 \times 5 \times 32$ & $1 \times 1$ & Same & Default \\
    \hline
    MaxPool & $2 \times 2$ & $2 \times 2$ & - & - \\
    \hline
    ReLU & - & - & - & - \\
    \hline
    Convolution & $5 \times 5 \times 64$ & $1 \times 1$ & Same & Default \\
    \hline
    MaxPool & $2 \times 2$ & $2 \times 2$ & - & - \\
    \hline
    ReLU & - & - & - & - \\
    \hline
    Flatten & - & - & - & - \\
    \hline
    Dense & $1024$ & - & - & Default \\
    \hline
    ReLU & - & - & - & - \\
    \hline
    Dense & $10$ & - & - & Default \\
    \hline
    Softmax & - & - & - & - \\
    \end{tabular}
    \end{center}
    \caption{MNIST and Fashion-MNIST Classifier Structure}
    \label{table:mnist-classifier-structure}
\end{table}
\begin{table}[H]
    \begin{center}
    \begin{tabular}{c | c | c | c | c }
    \hline \hline
    Layer & Kernel Size & Strides & Padding & Init \\
    \hline \hline
    Dropout & $0.2$ (drop rate) & - & - & - \\
    \hline
    Convolution & $3 \times 3 \times 96$ & $1 \times 1$ & Same & He \\
    \hline
    ReLU & - & - & - & - \\
    \hline
    Convolution & $3 \times 3 \times 96$ & $1 \times 1$ & Same & He \\
    \hline
    ReLU & - & - & - & - \\
    \hline
    Convolution & $3 \times 3 \times 96$ & $1 \times 1$ & Same & He \\
    \hline
    ReLU & - & - & - & - \\
    \hline
    MaxPool & $2 \times 2$ & $2 \times 2$ & - & - \\
    \hline
    Dropout & $0.5$ (drop rate) & - & - & - \\
    \hline
    Convolution & $3 \times 3 \times 192$ & $1 \times 1$ & Same & He \\
    \hline
    ReLU & - & - & - & - \\
    \hline
    Convolution & $3 \times 3 \times 192$ & $1 \times 1$ & Same & He \\
    \hline
    ReLU & - & - & - & - \\
    \hline
    Convolution & $3 \times 3 \times 192$ & $1 \times 1$ & Same & He \\
    \hline
    ReLU & - & - & - & - \\
    \hline
    MaxPool & $2 \times 2$ & $2 \times 2$ & - & - \\
    \hline
    Dropout & $0.5$ (drop rate) & - & - & - \\
    \hline
    Convolution & $3 \times 3 \times 192$ & $1 \times 1$ & Valid & He \\
    \hline
    ReLU & - & - & - & - \\
    \hline
    Convolution & $1 \times 1 \times 192$ & $1 \times 1$ & Same & He \\
    \hline
    ReLU & - & - & - & - \\
    \hline
    Convolution & $1 \times 1 \times 192$ & $1 \times 1$ & Same & He \\
    \hline
    ReLU & - & - & - & - \\
    \hline
    GlobalAvgPool & - & - & - & - \\
    \hline
    Dense & $10$ & - & - & Default \\
    \hline
    Softmax & - & - & - & - \\
    \end{tabular}
    \end{center}
    \caption{CIFAR10 allCNN Classifier Structure}
    \label{table:cifar-classifier2-structure}
\end{table}
\begin{table}[H]
    \begin{center}
    \begin{tabular}{ c | c | c | c } 
    \hline \hline
    Setting & MNIST & Fashion-MNIST & CIFAR10 \\
    \hline \hline
    Optimizer & Adam & Adam & Momentum \\
    Learning Rate & $1e^{-4}$ & 0.01 & 0.01 \\
    Learning Rate Decay & - & 0.1 & 0.1 \\
    Momentum & - & - & 0.9 \\
    Weight Decay & - & - & 0.001 \\
    Batch Size & 128 & 128 & 128 \\
    Shuffle & Yes & Yes & Yes \\
    Width Shift & - & - & 0.1 \\
    Height Shift & - & - & 0.1 \\
    Horizontal Flip & No & No & Yes \\
    Epoch & 80 & 80 & 350 \\
    \end{tabular}
    \end{center}
    \caption{Classifier Training Setting}
    \label{table:classifier-training}
\end{table}
\begin{table}[H]
    \begin{center}
    \begin{tabular}{c | c | c | c | c }
    \hline \hline
    Layer & Kernel Size & Strides & Padding & Init \\
    \hline \hline
    Dense & 32 & - & - & Default \\
    \hline
    ReLU & - & - & - & - \\
    \hline
    Dense & 64 & - & - & Default \\
    \hline
    ReLU & - & - & - & - \\
    \hline
    Dense & 32 & - & - & Default \\
    \hline
    ReLU & - & - & - & - \\
    \hline
    Dense & 1 & - & - & Default \\
    \hline
    Sigmoid & - & - & - & - \\
    \end{tabular}
    \end{center}
    \caption{Discriminator Structure}
    \label{table:discriminator-structure}
\end{table}
\begin{table}[H]
    \begin{center}
    \begin{tabular}{ c | c } 
    % \hline
    % \multicolumn{4}{c}{GanDef - Training} \\[0.5ex] 
    \hline \hline
    Setting & MNIST, Fashion-MNIST and CIFAR10 \\
    \hline \hline
    Optimizer & Adam \\
    Learning Rate & $1e^{-4}$ \\
    Batch Size & 128 \\
    Inner Epochs & 3 \\
    Shuffle & Yes \\
    $\gamma$ & 2 \\
    \end{tabular}
    \end{center}
    \caption{Discriminator Training Setting}
    \label{table:discriminator-training}
\end{table}

\end{appendices}
